# Supplementary material for: On Transforming Reinforcement Learning by Transformer: The Development Trajectory
Source: arXiv:2212.14164 source file (2023-01-20)
Supplement: Supplementary file 1 [file 7.Appendix.tex]

\appendices
\section{Proof of the First Zonklar Equation}
Appendix one text goes here.

% you can choose not to have a title for an appendix
% if you want by leaving the argument blank
\section{}
Appendix two text goes here.

\begin{abstract}

Transformer, originally devised for natural language processing, has also attested significant success in computer vision. Thanks to its super expressive power, researchers are investigating ways to deploy transformers to reinforcement learning (RL) and the transformer-based models have manifested their potential in representative RL benchmarks. In this paper, we collect and dissect recent advances on transforming RL by transformer (transformer-based RL or TRL), in order to explore its development trajectory and future trend. We group existing developments in two categories: architecture enhancement and trajectory optimization, and examine the main applications of TRL in robotic manipulation, text-based games, navigation and autonomous driving. For architecture enhancement, these methods consider how to apply the powerful transformer structure to RL problems under the traditional RL framework, which model agents and environments much more precisely than deep RL methods, but they are still limited by the inherent defects of traditional RL algorithms, such as bootstrapping and “deadly triad”. For trajectory optimization, these methods treat RL problems as sequence modeling and train a joint state-action model over entire trajectories under the behavior cloning framework, which are able to extract policies from static datasets and fully use the long-sequence modeling capability of the transformer. Given these advancements, extensions and challenges in TRL are reviewed and proposals about future direction are discussed. We hope that this survey can provide a detailed introduction to TRL and motivate future research in this rapidly developing field.
\end{abstract}
